# Supplementary material for: Temperature controlled motion of an antiferromagnet-ferromagnet interface within a dopant-graded FeRh epilayer
Source: arXiv:1412.7346 source file (2014-12-23)
Supplement: Supplementary file 1 [file Supplementary_Material.pdf]

# Temperature controlled motion of an antiferromagnet-ferromagnet interface within a dopant-graded FeRh epilayers

## Supplementary Material

### X-ray Reflectometry

The X-ray reflectometry (XRR) data were fitted using the GenX software[1]. The $FeRh_{1-x}X_x$ layer was broken up into three slabs, whilst the Al cap was assumed to be at least partly oxidised. Here X is the doping material (a mix of Pd and Ir), and *x* is the doping level. The parameters used to obtain the fit are given in Table S1 below. Interfacial width contains a quadrature addition of roughness and interfacial grading, which cannot be separated from specular reflectivity data alone.

**Table S1: X-ray reflectometry fitting parameters. *The MgO substrate was constrained to have the known bulk density and therefore there is no error bar on this parameter, since it was not varied in the fit.**

| Layer | Density (f.u./ Å$^3$) | Thickness (Å) | Interfacial Width (Å) |
|---|---|---|---|
| **$AlO_x$ cap** | 0.0376 ± 0.0007 | 60.7 ± 0.3 | 17.1 ± 0.3 |
| **$FeRh_{1-x}X_x$ top** | 0.0485 ± 0.0004 | 16.2 ± 0.5 | 26.6 ± 0.1 |
| **$FeRh_{1-x}X_x$ middle** | 0.04045 ± 0.00001 | 455 ± 4 | 18.0 ± 0.3 |
| **$FeRh_{1-x}X_x$ bottom** | 0.04053 ± 0.00006 | 54 ± 4 | 4 ± 4 |
| **MgO substrate** | 0.0436* | ∞ | 1.032± 0.005 |

### Scanning TEM-energy dispersive X-ray spectroscopy (STEM-EDX)

A constant profile of Fe and Rh concentration was observed in the epilayer.

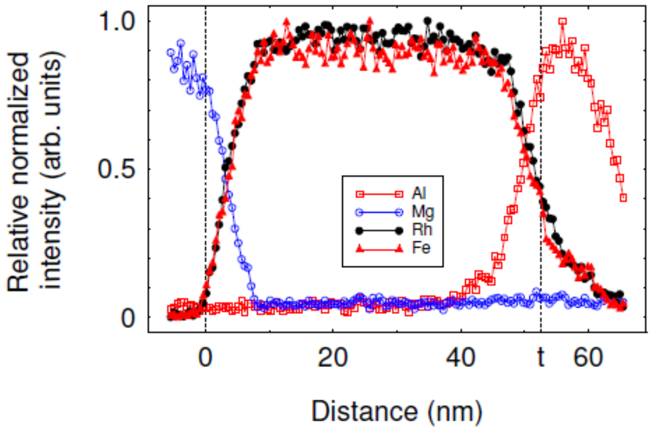


**Figure S1: The EDX determined profiles for the substrate-epilayer-cap.**

## Polarised Neutron Reflectivity (PNR)

The PNR data were modeled and fitted using Refl1D[2], which provides a thorough analysis of the confidence interval and parameter correlation using Bayesian statistics. To find a consistent set of starting conditions we fitted the data in pairs starting with $T$=175 °C and $T$=170 °C in the middle of the temperature range. This process produced an average chemical structure and a series of magnetic profiles. In each case the FeRh layer was split into two magnetic components with the total thickness and nuclear scattering length density constrained. At the end of the fitting process we inspected the resulting stable population and parameter correlation to determine if the fit had sufficiently converged. Other than the obvious correlations introduced by splitting the FeRh layer, all other parameters showed either weak or no correlations with the other fitting parameters. As a final step to confirm results, all the data sets were modeled together. Given these constraints the agreement is excellent. A single chemical profile (see Fig. S1) was enforced on all individual temperatures while the parameters associated with the shape of the *magnetic* profile were allowed to vary independently for each temperature. The chemical profile is consistent with the nominal SLD for each layer to within 10%. The chemical profile only differs significantly from the XRR established profile in the cap region. XRR is relatively insensitive to the light materials of the capping layer whereas the neutron measurement is not. The variation in SLD due to the dilute Pd, Ir doping is not modelled in the analysis as the effective change is below the sensitivity of our measurements. The profile extracted through the neutron measurement is consistent with the diffuse nature of the oxidized Al cap (Fig. 3(a)) as observed by TEM, though significantly broader than that established by the XRR. A summary of the PNR data and the resultant fits are shown in Fig S2. The PNR derived structural model is described in table S2. The large interfacial width relative to the layer thickness simply parameterizes the diffuse nature of the cap. The PNR derived magnetization data have been shifted by a small constant offset of 58 e.m.u./cm$^3$ in order to bring them into agreement with the SQUID results at the lowest measurement temperature.

**Table S2: Structural PNR parameters.**

| Layer | SLD ($\times 10^{-6}$/ Å$^2$) | Thickness (Å) | Interfacial Width (Å) |
|---|---|---|---|
| **$AlO_x$ cap** | 3.2 ± 0.8 | 66 ± 20 | 128 ± 40 |
| **$FeRh_{1-x}X_x$** | 6.2 ± 0.5 | 510 ± 10 | 26.6 ± 0.1 |
| **MgO substrate** | 6.5 ± 0.3 | ∞ | 5 ± 3 |

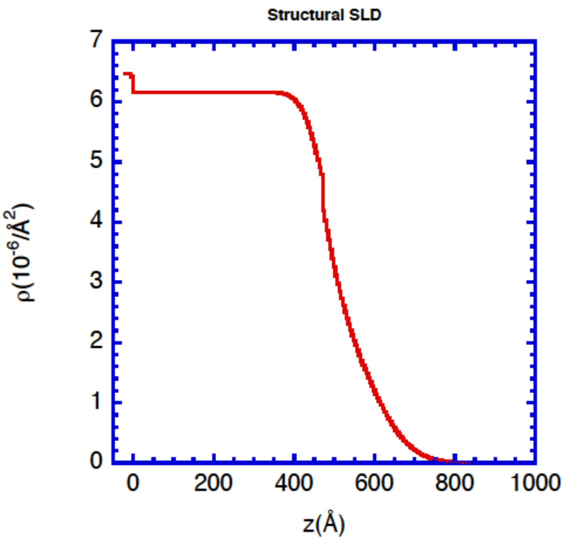


**Figure S2: The neutron scattering length density (SLD) profile used in the fitting of the PNR data.**

---

[1] M. Björck and G. Andersson, J. Appl. Cryst. **40**, 1174 (2007).

[2] http://www.reflectometry.org/danse/software.html
